# Supplementary material for: From Time-Invariant to Uniformly Time-Varying Control Barrier Functions: A Constructive Approach
Source: arXiv:2408.12964 source file (2024-08-23)
Supplement: Supplementary file 1 [file 30-appendix.tex]

\section*{Appendix}

\begin{proof}[Proof of Lemma~\ref{lemma:time-varying CBF without input constraints 1}]
	Before we start with the actual proof, we recall some important properties of convex functions which the proof is based on. At first, recall that for a convex function $ \alpha' $ it holds for all $ x,y\in\bbR $ that 
	\begin{align}
		\label{eq:time-varying CBF without input constraints 1 aux 00}
		\alpha'(\sigma x \!+\! (1\!-\!\sigma)y) \!\leq\! \sigma \alpha'(x) \!+\! (1\!-\!\sigma) \alpha'(y), \quad \!\sigma\!\in\![0,1].
	\end{align}
	For $ \sigma=1 $, this implies $ \alpha'(\sigma x) \leq \sigma \alpha'(x) $. Moreover, if additionally $ \alpha'(0)=0 $ (e.g., if $ \alpha' $ is a convex class~$ \calK $ function), then 
	$ \alpha' $ is superadditive for positive real numbers; that is, for all $ x,y\geq 0 $, it holds that
	\begin{align}
		\label{eq:time-varying CBF without input constraints 1 aux 0}
		\alpha'(x)+\alpha'(y) \leq \alpha'(x+y).
	\end{align}
	This can be shown as
	\begin{align*}
		\alpha'(x) &+ \alpha'(y) 
		= \alpha'\left( (x+y) \frac{x}{x+y} \right) + \alpha'\left( (x+y) \frac{y}{x+y} \right) \\
		&\leq \frac{x}{x+y} \alpha'(x+y) + \frac{y}{x+y} \alpha'(x+y) = \alpha'(x+y)
	\end{align*}
	where the inequality results from the fact that $ \alpha'(\sigma x) \leq \sigma \alpha'(x) $ for $ \sigma\in[0,1] $.
	
	Furthermore, we recall that the difference quotient $ D_{\alpha'}(x,y) := \frac{\alpha'(y)-\alpha'(x)}{y-x} $ of the convex function $ \alpha' $ is monotonously increasing in both of its arguments\footnote{This is a standard result and it can be easily shown as follows. At first, let $ x $ be fixed, and choose $ y = \sigma y' + (1-\sigma)x  $ where $ y'>x $; thus, $ y \leq y' $. Then, it follows that $ D(x,y) $ is monotonously increasing in~$ y $ as 
		\begin{align*}
			&D(x,y) = \frac{\alpha'(y)-\alpha'(x)}{y-x} = \frac{\alpha'(\sigma y' + (1-\sigma)x) - \alpha'(x)}{\sigma y' + (1-\sigma)x - x}  \\
			&\quad= \frac{\alpha'(\sigma y' + (1-\sigma)x) - \alpha'(x)}{\sigma y' - \sigma x}\stackrel{\eqref{eq:time-varying CBF without input constraints 1 aux 00}}{\leq} \frac{(1-\sigma)\alpha'(x) + \sigma \alpha'(y') - \alpha'(x)}{\sigma y' - \sigma x} \\
			&\quad= \frac{\alpha'(y')-\alpha'(x)}{y'-x} = D(x,y').
		\end{align*}
		The result follows for the first argument analogously. 
	}. Thus, we have $ \frac{\alpha'(y)-\alpha'(x)}{y-x} \leq \frac{\alpha'(y+c)-\alpha'(x+c)}{y-x} $ for all $ x<y $, $ c\geq 0 $, or equivalently,
	\begin{align}
		\label{eq:time-varying CBF without input constraints 1 aux 1}
		\alpha'(y)-\alpha'(x) \leq \alpha'(y+c)-\alpha'(x+c).
	\end{align}
	
	At last in addition to its convexity, we assume that $ \alpha' $ is an extended class~$ \calK_{e} $ function. Then, it holds for all $ \sigma \in [0,1/2] $, $ x\geq 0 $, that $ 0 \leq \alpha'((1-2\sigma)x) \leq \sigma \alpha'(-x)  + (1-\sigma) \alpha'(x) $ where the first inequality follows as $ \alpha' $ is class~$ \calK_{e} $ and thus it is non-negative for non-negative arguments; the second inequality follows from the convexity of $ \alpha' $. By rearranging terms, we obtain $ -\alpha'(x)\leq \sigma (\alpha'(-x)-\alpha'(x)) $, and thus for $ \sigma = 1/2 $ that for all $ x\geq 0 $ it holds
	\begin{align}
		\label{eq:time-varying CBF without input constraints 1 aux 2}
		-\alpha'(x)\leq\alpha'(-x).
	\end{align} 
	
	Now, we turn towards the actual proof of \eqref{eq:time-varying CBF without input constraints 1}. Therefore, let us define an extended version of $ \alpha_{2} $ as a convex extended class $ \calK_{e} $ function $ \alpha'_{2}: \bbR\rightarrow\bbR $ such that: (1) $ \alpha'_{2}(x) $ is an arbitrary continuous, convex and monotonously increasing continuation of $ \alpha_{2}(x) $ for all $ x<0 $; (2) $ \alpha'_{2}(x) = \alpha_{2}(x) $ for all $ x\in[0,A] $; and (3) $ \alpha'_{2}(x) = \alpha_{2}(A) + \alpha'_{1}(x-A) $ for all $ x\geq A $ where $ \alpha'_{1}(x) $ is some convex class~$ \calK $ function with $ \alpha'_{1}(x)\geq\alpha_{1}(x) $ for all $ x\geq0 $. 
	Next, we distinguish three cases, namely $ x_{1} \in [-A,0] $ with $ x_{1}+x_{2}\leq 0 $ (case~1a) and $ x_{1}+x_{2}\geq 0 $ (case~1b), and $ x_{1} \in [0,\infty) $ (case~2). Recall that $ x_{2}\in[0,A] $.
	
	\emph{Case~1a ($ x_{1} \in [-A,0] $ and $ x_{1}+x_{2}\leq0 $):} At first we note that since $ \alpha_{2} $ is convex it holds 
	\begin{align}
		\label{eq:time-varying CBF without input constraints 1 aux 3}
		\alpha_{2}(-(x_{1}+x_{2})) + \alpha_{2}(x_{2}) \stackrel{\eqref{eq:time-varying CBF without input constraints 1 aux 0}}{\leq} \alpha_{2}(-x_{1})
	\end{align}
	due to the superadditivity of $ \alpha_{2} $. Next, we consider the left-hand side of~\eqref{eq:time-varying CBF without input constraints 1}. By employing that $ \alpha_{1}(-x)\leq -\alpha_{2}(x) $ for all $ x\in[0,A] $ and that $ \alpha'_{2} $ is convex, we obtain
	\begin{align*}
		\alpha_{1}(x_{1}) \!+\! \alpha_{2}(x_{2}) \!&\leq\! -\alpha_{2}(-x_{1}) \!+\! \alpha_{2}(x_{2}) \!\stackrel{\eqref{eq:time-varying CBF without input constraints 1 aux 3}}{\leq}\! -\alpha_{2}(-(x_{1}\!+\!x_{2})) \\
		&= -\alpha'_{2}(-(x_{1}+x_{2})) \stackrel{\eqref{eq:time-varying CBF without input constraints 1 aux 2}}{\leq} \alpha'_{2}(x_{1}+x_{2}).
	\end{align*}
	Here we employed that $ -(x_{1}+x_{2})\in[0,A] $ in case~1a.
	
	\emph{Case~1b ($ x_{1} \in [-A,0] $ and $ x_{1}+x_{2}>0 $):} Noting that $ x_{1} + A \geq 0 $, we derive by starting again with the left-hand side of~\eqref{eq:time-varying CBF without input constraints 1} that
	\begin{align*}
		\alpha_{1}(x_{1}) \!\!+\!\! \alpha_{2}(x_{2}) \!&\leq\! -\alpha_{2}(-x_{1}) \!\!+\!\! \alpha_{2}(x_{2}) \!=\!  -\alpha'_{2}(-x_{1}) \!\!+\!\! \alpha'_{2}(x_{2}) \\ 
		\!&\stackrel{\eqref{eq:time-varying CBF without input constraints 1 aux 1}}{\leq}\! -\alpha'_{2}(-x_{1}\!+\!x_{1}\!+\!A) \!+\! \alpha'_{2}(x_{1}\!+\!x_{2}\!+\!A) \\
		&= -\alpha'_{2}(A) \!+\! \alpha'_{2}(x_{1}\!+\!x_{2}\!+\!A).
	\end{align*}
	
	\emph{Case~2 ($ x_{1} \in [0,\infty) $):} Recall that $ \alpha'_{2}(x) = \alpha_{2}(A) + \alpha'_{1}(x-A) $ for $ x\geq A $ with $ \alpha'_{1}(x)\geq\alpha_{1}(x) $ for all $ x\geq0 $. Thus, we have for $ x\geq 0 $ that
	\begin{align}
		\label{eq:time-varying CBF without input constraints 1 aux 4}
		\alpha_{1}(x) \leq \alpha'_{1}(x) = \alpha'_{2}(x+A) - \alpha_{2}(A).
	\end{align} 
	Furthermore by employing that $ \alpha'_{2} $ is convex, we obtain
	\begin{align*}
		\alpha_{1}(x_{1}) \!+\! \alpha_{2}(x_{2}) \!&\stackrel{\eqref{eq:time-varying CBF without input constraints 1 aux 4}}{\leq}\! - \alpha_{2}(A) \!+\! \alpha'_{2}(x\!+\!A) \!+\! \alpha_{2}(x_{2}) \\ 
		&= \alpha'_{2}(x\!+\!A) \!-\! \alpha'_{2}(A) \!+\! \alpha'_{2}(x_{2}) \\ &\stackrel{\text{\eqref{eq:time-varying CBF without input constraints 1 aux 0}}}{\leq} -\alpha'_{2}(A) \!+\! \alpha'_{2}(A\!+\!x_{1}\!+\!x_{2}).
	\end{align*}
	
	Summarizing cases~1a, 1b and~2, we choose $ \beta $ in~\eqref{eq:time-varying CBF without input constraints 1} as 
	\begin{align*}
		\beta(x_{1}\!+\!x_{2}) = \begin{cases}
			\alpha'_{2}(x_{1}\!+\!x_{2}) &\text{if } x_{1}\!+\!x_{2}\leq0,  \\
			-\alpha'_{2}(A)\!+\!\alpha'_{2}(x_{1}\!+\!x_{2}\!+\!A) &\text{if } x_{1} \!+\! x_{2}> 0.
		\end{cases}
	\end{align*}
	As shown, $ \beta $ satisfies~\eqref{eq:time-varying CBF without input constraints 1}. Moreover, $ \beta $ is continuous, it holds $ \beta(0) = 0 $, and $ \beta $ is monotonously increasing as $ \alpha'_{2} $ is class $ \calK_{e} $; thus, also $ \beta $ is class~$ \calK_{e} $. This concludes the proof.
\end{proof}

\begin{proof}[Proof of Lemma~\ref{lemma:time-varying CBF without input constraints 2}]
	The proof in the case of a concave function $ \alpha_{2} $ is more straightforward compared to the convex case. Before we start, we recall that the difference quotient $ D_{\alpha'}(x,y) := \frac{\alpha'(y)-\alpha'(x)}{y-x} $ of a concave function $ \alpha' $ is monotonously decreasing in both arguments. Thus, \eqref{eq:time-varying CBF without input constraints 1 aux 1} still holds, however only for non-positive $ c\leq 0 $. More precisely, it holds for all $ x<y $, $ c\leq 0 $ that
	\begin{align}
		\label{eq:time-varying CBF without input constraints 2 aux 1}
		\alpha'(y)-\alpha'(x) \leq \alpha'(y+c)-\alpha'(x+c).
	\end{align}
	
	Now, we turn towards the actual proof of~\eqref{eq:time-varying CBF without input constraints 2}. To this end, we define again an extended version of $ \alpha_{2} $, however this time as a concave extended class $ \calK_{e} $ function $ \alpha'_{2}:\bbR\rightarrow\bbR $ such that $ \alpha'_{2}(x)=\alpha_{2}(x) $ for all $ x\geq 0 $. Next, we distinguish two cases, namely $ x_{1}\in[-A,0] $ (case~1) and $ x_{1}\in[0,\infty) $ (case~2). Recall that $ x_{2}\in[0,A] $.
	
	\emph{Case 1 ($ x_{1}\in[-A,0] $):} Consider the left-hand side of~\eqref{eq:time-varying CBF without input constraints 2}. By employing that $ \alpha_{1}(-x)\leq -\alpha_{2}(x) $ for all $ x\in[0,A] $ and that $ \alpha'_{2} $ is concave, we obtain
	\begin{align*}
		\alpha_{1}(x_{1}) \!&+\! \alpha_{2}(x_{2}) \!\leq\! -\alpha_{2}(-x_{1}) \!\!+\!\! \alpha_{2}(x_{2}) \!=\! -\alpha'_{2}(-x_{1}) \!\!+\!\! \alpha'_{2}(x_{2}) \\
		&\stackrel{\eqref{eq:time-varying CBF without input constraints 2 aux 1}}{\leq} -\alpha'_{2}(-x_{1} \!+\! x_{1}) \!+\! \alpha'_{2}(x_{1}\!+\!x_{2}) = \alpha'_{2}(x_{1}\!+\!x_{2})
	\end{align*}
	where the last inequality is obtained by adding $ c=x_{1} $, which is non-positive by assumption, to the arguments of $ \alpha'_{2} $. For the case that $ x_{1} + x_{2}\geq 0 $, we note that the right-hand side is upper-bounded by
	\begin{align*}
		\alpha'_{2}(x_{1}+x_{2}) \leq \alpha_{1}(x_{1}+x_{2})+\alpha'_{2}(x_{1}+x_{2}).
	\end{align*}
	This observation is needed later on for the construction of the extended class~$ \calK_{e} $ function~$ \beta $.
	
	\emph{Case 2 ($ x_{1}\in[0,\infty) $):}  In this case, it always holds that $ x_{1}+x_{2}\geq 0 $. Thus, we directly obtain 
	\begin{align*}
		\alpha_{1}(x_{1}) \!+\! \alpha_{2}(x_{2}) &= \alpha_{1}(x_{1}) \!+\! \alpha'_{2}(x_{2}) \\
		&\leq \alpha_{1}(x_{1}\!+\!x_{2}) \!+\! \alpha'_{2}(x_{1}\!+\!x_{2}).
	\end{align*}
	
	Summarizing cases~1 and~2, we choose $ \beta $ in~\eqref{eq:time-varying CBF without input constraints 2} as
	\begin{align*}
		\beta(x_{1}\!+\!x_{2}) = 
		\begin{cases}
			\alpha'_{2}(x_{1}\!+\!x_{2}) &\text{if } x_{1}\!+\!x_{2}< 0, \\
			\alpha_{1}(x_{1}\!+\!x_{2}) \!+\! \alpha'_{2}(x_{1}\!+\!x_{2}) &\text{if } x_{1}\!+\!x_{2}\geq 0.
		\end{cases}
	\end{align*}
	As shown, $ \beta $ satisfies~\eqref{eq:time-varying CBF without input constraints 2}. Moreover, $ \beta $ is continuous, it holds $ \beta(0) = 0 $, and $ \beta $ is monotonously increasing as both $ \alpha_{1} $ and $ \alpha_{2}' $ are class $ \calK_{e} $ functions; thus, also $ \beta $ is a class~$ \calK_{e} $ function. This result even holds for $ A\rightarrow\infty $, as the construction of $ \beta $ does not rely on $ A $. This concludes the proof.
\end{proof}
